# Supplementary material for: Dynamical instabilities in disc-planet interactions
Source: arXiv:1203.4829 source file (2012-03-21)
Supplement: Supplementary file 2 [file appendix1.tex]

\section{Parameterisation of disc models for the vortex instability}\label{Qo_Md}
Disc models used to study the vortex instability are labelled by $Q_o$, 
which corresponds to values of $Q_p$ and disc-to-star mass ratio
given in Table  
\ref{Qo_Md_conversion}.  

\begin{table}
  \centering
  \caption{Relationship between the initial Keplerian Toomre stability
    parameter at the outer boundary, $Q_o$, at the planet's initial
    orbital radius, $Q_p$, and the disc-to-star mass ratio, for disc models used  in disc-planet interactions. }
  \begin{tabular}{ccc}
    \hline
    $Q_o$ & $Q_p$ & $M_d/M_*$ \\
    \hline\hline
    1.5 & 2.62 & 0.063 \\
    2.0 & 3.49 & 0.047 \\
    2.5 & 4.36 & 0.038 \\
    3.0 & 5.23 & 0.031 \\
    3.5 & 6.11 & 0.027 \\
    4.0 & 6.98 & 0.024 \\
    8.0 & 14.0 & 0.012 \\
    \hline
  \end{tabular}
  \label{Qo_Md_conversion}
\end{table}

\section{Artificial vortices in an accretion disc}\label{kidasetup}
The artificial Kida-like vortices used in \S\ref{hydro2} are setup as follows.
Consider a small patch of the disc, whose centre $(r_p, \varphi_p)$
rotates at angular speed $\Omega_p$ about the primary and set up local
Cartesian co-ordinates $x=r_p(\varphi-\varphi_p),\,y=r_p-r$. In the $(x,y)$
frame, there exists a Kida vortex solution for incompressible flow,
whose velocity field

$(u_x, u_y)$ is
\begin{align}  
   u_x = \frac{3\Omega_p\zeta y}{2(\zeta -1)},\quad
   u_y = -\frac{3\Omega_p x}{2\zeta(\zeta-1)}
\end{align}
inside the vortex core.  The ratio of the vortex
semi-major to semi-minor axis being  $\zeta=a/b$ is a free
parameter.  This velocity field is such that the
 vorticity $\omega$ is constant in the rotating frame. The elliptical boundary of the vortex
is defined such that
 $\omega =-3\Omega_p(1+\zeta^2)/(2\zeta(\zeta-1)) = \omega_v - 3\Omega_p/2 $ inside the
boundary  of the vortex and $\omega = - 3\Omega_p/2$ outside. The quantity
 $\omega_v= -3\Omega_p(1+\zeta)/(2\zeta(\zeta-1))$ is then
the vorticity of the vortex core relative to the background.
Being negative, this corresponds to an anticyclonic vortex.
In order to introduce perturbations corresponding
to Kida vortices,  we impose perturbations $\dd u_r \equiv
-v_y,\,\dd u_\varphi \equiv  v_x$ inside a specified elliptical boundary with an  exponential decay
outside. The boundary is fixed  by specifying  $\zeta = 8$
and its  semi-major axis $a=H(r_p)$ where the  reference radius is
$r_p=1$.

\section{Mutual horseshoe turns in the shearing sheet}\label{horseshoe}
We describe the gravitational interactions between two vortices in the
shearing sheet. It is assumed they behave like point masses and that
pressure forces may be neglected. We indicate below why this is a
reasonable assumption.

Consider a local Cartesian co-ordinate system $(x,y)$ that co-rotates
with a small patch of fluid  with angular velocity  $\Omega$ about the
primary, at a distance $r_p$. We have
$x=r-r_p,\,y=r_p(\varphi - \Omega 
t)$. Let $(x_j,y_j)$ denote the co-ordinates of the  centroid of  the $j^\mathrm{th}$
vortex  and $m_j$ be its  mass $(j = 1 , 2).$  Defining
$X\equiv x_2 - x_1,\,Y \equiv y_2 - y_1$ and $\mathcal{M} \equiv
m_2+m_1$, the equations of motion give 
\begin{align}
 & \ddot{X} - 2\Omega\dot{Y} = 3\Omega^2X - \frac{G\mathcal{M}X}{R^3},\\
 & \ddot{Y} + 2\Omega\dot{X} =  - \frac{G\mathcal{M}Y}{R^3},
\end{align}
where $R^2\equiv X^2 + Y^2$. 
%It is straight forward to show that $X$
%relates to the $x$-motion of $m_1$ relative to the centre of mass of
%the two-vortex system, and similarly for $Y$. We can think of these
%equations as describing the motion of $m_1$ about a mass $\mathcal{M}$
%held fixed. 
These equations imply the constancy  of the Jacobi constant
\begin{align}
  J \equiv \frac{1}{2}\left( \dot{Y}^2 + \dot{X}^2\right) -
  \frac{3}{2}\Omega^2 X^2 - \frac{G\mathcal{M}}{R}.
\end{align}
  Let the  initial conditions be $X=
X_0,\,Y=\infty,\,\dot X=0,\,\dot Y = -3\Omega X_0/2.$ We assume the point of
closest approach occurs when  $X=\dot{Y}=0$. Equating $J$  at the initial time  and
at the time of closest approach we obtain
\begin{align}
  -\frac{3}{8} \Omega^2 X_0^2 = \frac{1}{2}\dot{X}^2 - \frac{G\mathcal{M}}{Y}
\label{Jacobi}
\end{align}
at the time of closest approach.
Since the vortices are then  at minimum separation, $\ddot{Y}>0$.
 The $y$  component of the equation of motion then  implies
\begin{align}
  \frac{1}{2}\dot{X}^2 > \frac{1}{8}\left(\frac{G\mathcal{M}}{\Omega Y^2}\right)^2.
\end{align}
Substituting $\dot X$ from  (\ref{Jacobi})  the inequality becomes 
\begin{align}\label{min_sep1}
\frac{3}{8}\hat{X}_0^2  < \frac{q}{\hat{Y}} - \frac{q^2}{8\hat{Y}^4}  
\end{align}
at minimum separation, where $\hat{X}_0 = X_0/r_p$, $\hat{Y} =
Y/r_p$, $q=\mathcal{M}/M_*$ and we have assumed $\Omega^2 =
GM_*/r_p^3$.

% Inserting data from Fnsg, $X_0 = 7.1\times10^{-3},\, r_p = 0.985,\, q
% = 7\times 10 $ implies that $0.4H<Y<73H$ which does not provide
% a useful constraint on the minimum separation, and the upper limit is
% well beyond the validity of the shearing sheet. However, note that the
% same upper limit is obtained, had we balanced the terms $-2\Omega
% \dot{Y}$ and $3\Omega^2 X$ in the $x$ equation of motion and used this
% in the $y$ equation. 
Eq. \ref{min_sep1} is useful for the case there vortices are just able
to undergo U turns. For fixed $q$, the function
\begin{align}\label{fy}
  f(\hat{Y};q) = \frac{q}{\hat{Y}} - \frac{q^2}{8\hat{Y}^4}
\end{align}
has a maximum value at $\hat{Y} = (q/2)^{1/3},$
corresponding to the
maximum conceivable  initial separation $X_0=X_s,$ where
\begin{align}\label{xs}
  X_s = 2^{2/3}q^{1/3}r_p.
\end{align}
If $X_0>X_s$ then equation (\ref{min_sep1})  cannot be satisfied and there
can be no horseshoe turns. For initial separations  $X_0<X_s$, (\ref{min_sep1})
implies that  the
minimal inter-vortex distance must exceed  $q^{1/3}/2$ (so that $f>0$). 
Now for sufficiently large $q,$ $q^{1/3}/2$ will be larger
than the critical separation  for merging, 
so merging is avoided during the  encounter.  

It is interesting to compare equation (\ref{xs})  to the estimate of the horseshoe
half-width $x_s$ of  \cite{paardekooper09}. They found $x_s=
1.68(q/h)^{1/2}r_p$ based on hydrodynamic simulations for low mass
planets. Equating $x_s$ and $X_s$
with $h=0.05$ we find $q=8.9\times10^{-5}.$
This should give the minimum $q$ for which pressure effects
could be ignored.
 Inserting
this value in  \cite{murray00}'s model of co-orbital satellites
gives a minimal separation of $0.58$ (see the estimate in
\S\ref{vortices_planets}), close to simulation results.   
Hence, if the vortex-pair interaction is purely gravitational, a
single vortex behaves in a similar way to  $\sim 15$ Earth masses, i.e. a low-mass
protoplanet.

Considering a vortex size of order $H$, the vortex-to-star mass ratio
is $q\sim \pi H^2\Sigma/M_*\simeq h^3/Q$. For a self-gravitating vortex where
$Q\sim 1$ we have $q\simeq h^3=1.25\times10^{-4}$ for $h=0.05$,
slightly exceeding the threshold value above.
Hence we expect the pressureless treatment of self-gravitating
vortex-vortex interactions to be acceptable for the purpose 
of explaining the resisted-merging of self-gravitating vortices. 

%Inserting $q=7\times10^{-5}$ gives $X_s \simeq
%0.065r_p$. Coincidentally, this is close to the hydrodynamic estimate by
%\cite{paardekooper09} who found that the horseshoe half-width $x_s$
%associated with low-mass planets is $x_s =
%1.68\sqrt{q/h}r_p$. Inserting $q=7\times10^{-5}$ and $h=0.05$ (as
%adopted in simulations here) gives $x_s = 0.063r_p$. Both values
% corresond to $1.3H$. Thus, vortices of size $H$
%may still merge. % if they are on horseshoe orbits with maximal initial

% separation and their separation at closest approach is still less than
% critical for merging ($\sim 3H$ for a vortex size $H$). 

% ------------------------------------------------------------------------

%%% Local Variables: 
%%% mode: latex
%%% TeX-master: "../thesis"
%%% End: 
