# Supplementary material for: Dynamical instabilities in disc-planet interactions
Source: arXiv:1203.4829 source file (2012-03-21)
Supplement: Supplementary file 4 [file appendix1.tex]

\section{Upper limit on the horseshoe width}\label{xslimit}

\indent We deduce an upper limit on the horseshoe width $x_s$  that is valid  in the limit
of  either zero  or constant pressure. Consider a local Cartesian
frame that  has origin at the planet and hence co-rotates with it with the Keplerian
angular velocity
$\Omega_p =\sqrt{GM_*/r_p^3}.$ Here $M_*$ is the mass of the central object and
$r_p$ is the orbital radius of the planet.
In this frame  fluid elements approach the
planet from $(x=x_0>0,\,y=\infty)$ with velocity $(0,-3\Omega_px_0/2).$
 Suppose such a fluid element  executes a horseshoe
turn crossing the co-orbital radius  at $q=(0,y)$ with velocity $(v_x,0)$.

 We wish to
determine an upper bound on the value of $x_0$  for which such motion occurs.
 The  equation of motion governing a fluid element or particle is
\begin{align}\label{horseshoe}
\frac{D\mathbf{v}}{Dt}+2\Omega_p\hat{\mathbf{z}}\wedge\mathbf{v} = 
 -\nabla\Phi_\mathrm{eff}, 
\end{align}
where
\begin{align}
 \Phi_\mathrm{eff}= -\frac{GM_p}{\sqrt{x^2+y^2}}-\frac{3}{2}\Omega_p^2x^2.
\end{align}
Here the {\it effective potential} $ \Phi_\mathrm{eff}$  contains contributions from the gravitational
potential of the planet of mass $M_p$ and  the tidal potential associated with
the central object.

From  equation  (\ref{horseshoe}) it follows that  the Jacobi invariant  
\begin{align}\label{jacobi}
J = \frac{1}{2}\mathbf{v}^2 + \Phi_\mathrm{eff}
\end{align}
is constant along a particle path. Equating $J$  evaluated at $(x,y)=(x_0,\infty)$
to $J$ evaluated at  $q$
gives
\begin{align}\label{eq1}
-\frac{3}{8}\Omega_p^2x_0^2 = \frac{1}{2}v_x^2 -\frac{GM_p}{y}.
\end{align}
The steady-state Euler equation of motion for $v_y$ evaluated at $q$ is
\begin{align}\label{eq2}
v_{x}\p_x v_y +2\Omega_p v_x = -GM_p/y^2.
\end{align}
Since in the neighbourhood of $q$ for the type of  streamline
we consider,  $v_x<0$ and    $ \p_x v_y<0$ we deduce that
\begin{align}\label{vxlimit}
|v_x|>\frac{GM_p}{2\Omega_p y^2}.
\end{align}
Combining equation  (\ref{eq1}) and equation  (\ref{vxlimit}) we find that
\begin{align}\label{limit}
-\frac{3}{8}\Omega_p^2x_0^2 > \frac{1}{2}\left(\frac{GM_p}{2\Omega_p y^2}\right)^2
 -\frac{GM_p}{y}.
\end{align}
Writing $x_0 = \hat{x}_0 r_h,$ where the Hill radius $r_h = (M_p/(3M_*))^{1/3}r_p$ and
similarly  setting $y = \hat{y} r_h $, we obtain
\begin{align}
  \hat{x}_0 < \sqrt{\frac{8}{\hat{y}} - \frac{3}{\hat{y}^4}} \lesssim 2.3.
\end{align}
Thus because  the maximum possible  value of the right hand side of the above is $2.3,$
we deduce that  particles executing a U-turn could not have originated
further than $2.3r_h.$ This is comparable to the value of $2.5r_h$ 
that has been estimated from hydrodynamic simulations \citep{artymowicz04b,paardekooper09}.
% ------------------------------------------------------------------------

%%% Local Variables: 
%%% mode: latex
%%% TeX-master: "../thesis"
%%% End: 
